# Supplementary material for: Improving Accuracy of Electrochemical Capacitance and Solvation Energetics in First-Principles Calculations
Source: arXiv:1801.07705 source file (2018-03-30)
Supplement: Supplementary file 1 [file SI.pdf]

# Supplementary information for "Improving Accuracy of Electrochemical Capacitance and Solvation Energetics in First-Principles Calculations"

Ravishankar Sundararaman,[1, a] Kendra Letchworth-Weaver,[2] and Kathleen Schwarz[3, b]
[1] *Department of Materials Science and Engineering, Rensselaer Polytechnic Institute, Troy, NY 12180*
[2] *Center for Nanoscale Materials, Argonne National Laboratory, Argonne, IL, 60439*
[3] *National Institute of Standards and Technology, Material Measurement Laboratory, Gaithersburg, MD, 20899*

## I. CONVERGENCE CHECKS

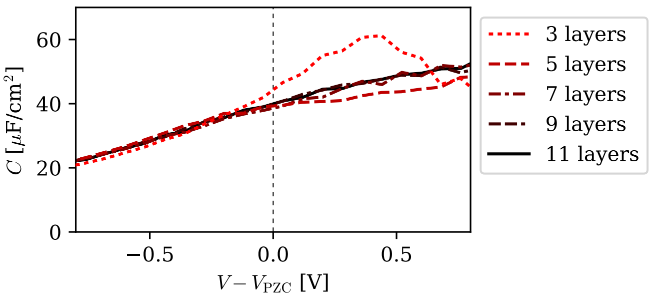


FIG. 1. Refit NonlinearPCM[1] capacitance of Ag(100) with 1 M electrolyte as a function of number of slab layers. Size-converged capacitance results are obtained for 7 atomic layers.

All Ag(100) electrochemical capacitance calculations shown in the main text use 7 layer slabs, $12 \times 12 \times 1$ $k$-point sampling and cold smearing with width $\sigma = 0.01\ E_h$. Figure 1 shows the variation of the predicted capacitance with number of layers, using the refit NonlinearPCM[1] model as an example. The capacitance is converged to $\sim 1\%$ accuracy with 7 layers, which we use in the main text results. In contrast, the 5-layer slab results incur $> 10\%$ errors, while the 3-layer slab exhibits qualitatively incorrect behavior with a misleading capacitance hump.

Figure 2 shows the variation of the predicted capacitance of the 7-layer Ag slab with $k$-point sampling ($N_k \times N_k \times 1$) and smearing width ($\sigma$), once again using the refit NonlinearPCM[1] model as an example. The results for $N_k = 12$ are converged within 1 % of those with finer $k$-point sampling, $N_k = 24$, at fixed smearing width $\sigma = 0.01\ E_h$. The results for smearing width $\sigma = 0.01\ E_h$ are, in turn, converged within 1 % of those with lower smearing width $\sigma = 0.005\ E_h$ at fixed $N_k = 24$. Consequently, $N_k = 12$ and $\sigma = 0.01\ E_h$ used in the main text results are converged to within 1% with respect to both $k$-points and smearing.

[a] Electronic mail: sundar@rpi.edu
[b] Electronic mail: kas4@nist.gov

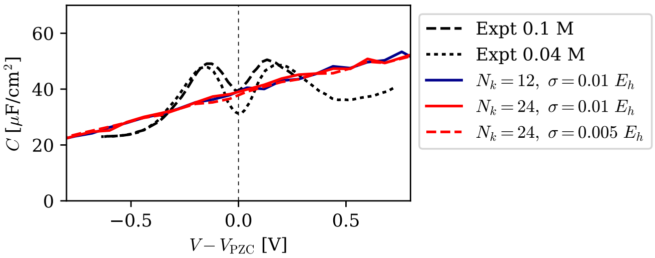


FIG. 2. Refit NonlinearPCM capacitance of 7-layer Ag(100) with 1 M electrolyte for different numbers of $k$-points per dimension, $N_k$, and smearing widths, $\sigma$. Calculations with $N_k = 12$ and $\sigma = 0.01\ E_h$ produce identical results to larger $N_k$ and smaller $\sigma$, indicating that they are comverged.

## II. CANDLE CAPACITANCE

The CANDLE solvation model[2] adjusts the size of its dielectric cavity based on the solute electric field to capture asymmetry in solvation of cations and anions, which allows it to exhibit the best overall accuracy for solvation energies within a single parametrization (as shown in Table 2 of the main text as well as Table II below). However, this results in a lower capacitance for positively charged surfaces and a higher value for negatively charged ones, and an unphysical spike at field strengths where the cavity changes size, as shown in Figure 1 of the main text.

Figure 3 explores this unphysical spike in the capacitance further and shows that it in fact also depends on the unit cell size. This is because the CANDLE cavity accounts for the asymmetry by including a dependence on the solute electric field. This electric field is well-defined and unit-cell independent for neutral molecules as well as charged ions when Coulomb truncation[3] is used. However, for slab geometries, even with Coulomb truncation, the potential diverges logarithmically for charged slabs and results in electric fields that converge very slowly $\sim 1/L_z$, with unit cell length $L_z$ along the truncated slab normal direction. (Figure 1 in the main text uses $L_z = 70$ Å.) The corresponding effect on the charging curve Figure 3(b) is less severe; it is the derivative with potential in the differential capacitance that amplifies the effect of the cavity transition and generates the observed spike. Additionally, this effect cancels in energy differences between systems at the same potential, which is the relevant quantity for evaluating reaction mechanisms. Therefore the CANDLE solvation model remains accurate for electrocatalysis[4] *despite* this issue in the differential capacitance.

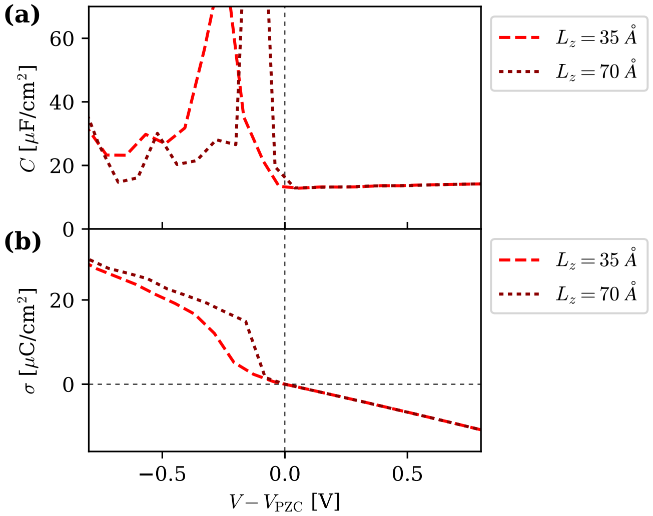


FIG. 3. (a) CANDLE[2] capacitance of 7-layer Ag(100) with 1 M electrolyte as a function of unit cell length $L_z$, and (b) corresponding surface charge density. The solute electric-field dependence of CANDLE introduces an unphysical unit-cell dependent differential capacitance, which has a smaller effect on the charging curve and hence the energies.

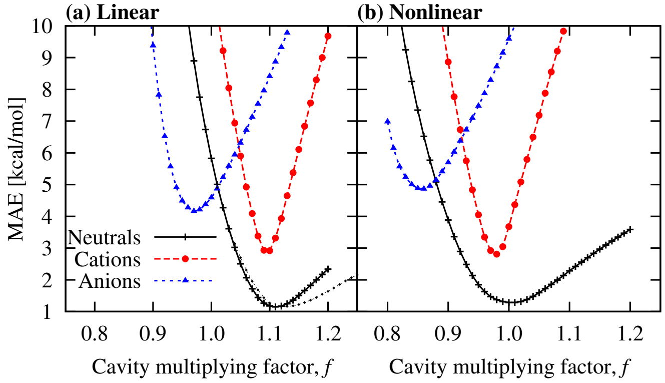


FIG. 4. Mean absolute error (MAE) for aqueous solvation energies of 240 neutral molecules, 51 cations and 55 anions for the (a) linear and (b) nonlinear soft-sphere solvation model. Cavity surface tension $t$ is held constant at the optimized values, $9.67 \times 10^{-6}$ $E_h/a_0^2$ for the linear and $1.02 \times 10^{-5}$ $E_h/a_0^2$ for the nonlinear model. The dotted line shows the MAE of the original soft-sphere model for 13 neutral molecules reported in Ref. 5 for comparison. Note that anions require smaller cavities than cations and neutral molecules due to charge asymmetry of hydration, and that the nonlinear model requires overall smaller cavities to compensate for saturation of the dielectric response.

## III. NESS PARAMETRIZATION DETAILS

The Nonlinear Electrochemical Soft-Sphere (NESS) solvation model incorporates the cavity definition of the Soft-Sphere model[5] into the NonlinearPCM[6] model. It retains the definitions for the nonlinear dielectric and ionic responses as well as the effective surface tension term for non-electrostatic solvation energy contributions, exactly as in Ref. 6, as discussed in the main text.

| Model / Variant | | $f$ | $t$ $[E_h/a_0^2]$ |
|---|---|---|---|
| Original[5] soft-sphere | Neutrals | 1.16 | $7.39 \times 10^{-6}$ |
| | Cations | 1.10 | |
| | Anions | 1.00 | |
| Linear soft-sphere | Neutrals | 1.11 | $9.67 \times 10^{-6}$ |
| | Cations | 1.10 | |
| | Anions | 0.97 | |
| Nonlinear soft-sphere | Neutrals | 1.00 | $1.02 \times 10^{-5}$ |
| | Cations | 0.98 | |
| | Anions | 0.86 | |

TABLE I. Fit parameters for the original[5] soft-sphere continuum solvation model, and the refit linear and nonlinear response versions. Small differences in the optimum parameters between Ref. 5 and the present linear version may arise from wavelet norm-conserving versus plane-wave ultrasoft basis - pseudopotential combinations, and grid versus plane-wave implementations of the electrostatics.

| Model / variant | | MAE [kcal/mol] | | | |
|---|---|---|---|---|---|
| | | Neutral | Cations | Anions | All |
| **Linear dielectric** | | | | | |
| LinearPCM[6]=VASPsol[7] | | 1.27 | 2.10 | 15.1 | 3.59 |
| SCCS[8,9] | Neutrals | 1.20 | 2.55 | 17.4 | 3.97 |
| | Cations | – | 2.26 | – | – |
| | Anions | – | – | 5.54 | – |
| CANDLE[2] | | 1.27 | 2.62 | 3.46 | **1.81** |
| Original[5] soft-sphere | Neutrals | 1.25 | 6.02 | 10.4 | 3.41 |
| | Cations | 1.46 | 2.88 | 7.82 | 2.68 |
| | Anions | 6.56 | 12.6 | 4.38 | 7.10 |
| Linear soft-sphere | Neutrals | 1.15 | 3.32 | 8.87 | 2.69 |
| | Cations | 1.18 | 2.92 | 8.41 | 2.58 |
| | Anions | 8.90 | 17.4 | 4.16 | 9.39 |
| **Nonlinear dielectric** | | | | | |
| Orig. NonlinearPCM[6] | | 1.28 | 16.1 | 27.0 | 7.55 |
| Refit NonlinearPCM[1] | | 1.44 | 14.4 | 27.6 | 7.51 |
| Nonlinear soft-sphere (NESS) | Neutrals | 1.29 | 3.67 | 9.58 | 2.96 |
| | Cations | 1.37 | 2.81 | 8.72 | 2.75 |
| | Anions | 6.51 | 14.6 | 4.86 | 7.44 |

TABLE II. Comparison of mean absolute errors (MAEs) in aqueous solvation energies of the same set of 240 neutral molecules, 51 cations and 55 anions between several prominent grid / plane-wave based solvation models. CANDLE yields the lowest MAE in a single parametrization due to charge-asymmetry correction, but that leads to unphysical features in the capacitance (Figure 3). The NESS model parametrized to neutral solvation energies is reasonably accurate for solvation energies (highlighted below), while simultaneously predicting electrochemical capacitance in good agreement with experiment (Figure 3 in main text).

The resulting model has two empirical parameters, the cavity scale factor $f$, and the effective tension $t$ ($= \alpha + \gamma$ in Ref. 5's notation), which we fit to the solvation free energies of a large set of neutral solutes, cations and anions as indicated in Figure 4. Table I shows the optimized parameters and Table II compares the accuracy of solvation energies for neutral solutes, cations and anions in several solvation models. Results for the linear version of the model, effectively identical to Ref. 5 except for the basis set and pseudopotentials, agree very well with the results from Ref. 5, providing a check on the implementation.

Our new NESS model performs comparably to the linear

Soft-Sphere model, and in its parametrization to neutral solutes, is substantially more accurate than the original NonlinearPCM.[6] It still falls short of CANDLE,[2] which is able to deliver the best overall accuracy for solvation free energies within a single parametrization because it accounts for charge asymmetry. However, that feature of CANDLE results in unphysical capacitance predictions, as shown in Figure 3 and discussed above.

## REFERENCES

[1]R. Sundararaman and K. Schwarz, J. Chem. Phys. **146**, 084111 (2017).
[2]R. Sundararaman and W. Goddard, J. Chem. Phys **142**, 064107 (2015).
[3]R. Sundararaman and T. Arias, Phys. Rev. B **87**, 165122 (2013).
[4]H. Xiao, T. Cheng, W. A. Goddard III, and R. Sundararaman, J. Am. Chem. Soc. **138**, 483 (2016).
[5]G. Fisicaro, L. Genovese, O. Andreussi, S. Mandal, N. N. Nair, N. Marzari, and S. Goedecker, J. Chem. Theory Comput. **13**, 3829 (2017).
[6]D. Gunceler, K. Letchworth-Weaver, R. Sundararaman, K. A. Schwarz, and T. A. Arias, Modell. and Simul. Mat. Sci. Eng. **21**, 074005 (2013).
[7]K. Mathew, R. Sundararaman, K. Letchworth-Weaver, T. A. Arias, and R. G. Hennig, J. Chem. Phys. **140** (2014).
[8]O. Andreussi, I. Dabo, and N. Marzari, J. Chem. Phys **136**, 064102 (2012).
[9]C. Dupont, O. Andreussi, and N. Marzari, J. Chem. Phys **139**, 214110 (2013).
